# Supplementary material for: NAAQA: A Neural Architecture for Acoustic Question Answering
Source: arXiv:2106.06147 source file (2024-01-12)
Supplement: Supplementary file 1 [file appendix.tex]

\onecolumn
\begin{center}
    \Huge Supplementary Material
\end{center}

\noindent
This document contains supplementary material to the paper "NAAQA: A Neural Architecture for Acoustic Question Answering". Some of the cross-references will refer to the main paper.
%JR \jean{see: \href{https://journals.ieeeauthorcenter.ieee.org/create-your-ieee-journal-article/prepare-supplementary-materials}{supplementary material link}}
\section{Detailed training settings}
\label{appendix:training_settings}
All models were trained for a maximum of 40 epochs or until the validation loss stops decreasing for 6 consecutive epochs. 
The Adam optimizer \cite{adam2015} with a learning rate of \num{3e-4} was used to optimize the cross entropy loss. 
To reduce the likelihood of the model getting trapped in a local minima, the learning rate is automatically reduced by a 0.1 factor if the validation loss stops decreasing for 3 consecutive epochs.
L2 regularization with a weight decay of \num{5e-6}, dropout~\cite{srivastava14a} with a drop probability of 0.25 and batch normalization~\cite{IoffeAndSzegedy2015ICMLConditionalBatchNormalization} are used to regularize the learning process. 
A batch size of 128 is used for all experiments. 
The following 5 random seeds were used to run all experiments : 
\emph{876944 189369 682421 175326 427438}

\section{Time and Frequency coordinate maps impact}
\label{appendix:coordinate_maps}

\begin{table}[H]
    \centering
    \resizebox{\textwidth}{!}{
        \begin{tabular}{ccccccccccccc}
            \hline
            \hline
			 			          & \multicolumn{12}{c}{Accuracy by question type on the test set (\%)} \\
			Coordinate       &     &            &      &            &          &       & Absolute & Global   & Relative &       & Count      & Count  \\
			Maps      & Overall & Instrument & Note & Brightness & Loudness & Exist & Position & Position & Position & Count & Comparison & Instruments \\
            \hline
Time only & \textbf{79.0 ±0.43} & \textbf{80.8 ±1.22} & \textbf{73.0 ±0.84} & \textbf{90.8 ±0.52} & 86.8 ±0.49 & 80.2 ±0.75 & \textbf{80.2 ±0.89} & \textbf{89.0 ±0.60} & 53.1 ±0.90 & 52.1 ±0.70 & \textbf{61.1 ±0.56} & \textbf{49.3 ±0.47} \\
Time \& Freq & 78.7 ±0.70 & 80.3 ±0.92 & 72.5 ±0.82 & 90.8 ±0.83 & \textbf{87.0 ±1.02} & \textbf{80.6 ±0.47} & 79.9 ±1.25 & 88.9 ±0.58 & \textbf{54.8 ±1.21} & \textbf{52.9 ±0.42} & 59.1 ±2.46 & 46.0 ±3.14 \\
None & 63.8 ±0.70 & 73.3 ±0.72 & 61.8 ±0.62 & 87.6 ±0.66 & 84.6 ±0.96 & 77.1 ±0.56 & 41.0 ±2.19 & 69.8 ±1.33 & 49.0 ±2.02 & 45.9 ±0.80 & 59.3 ±0.41 & 44.6 ±1.71 \\
Freq only & 61.7 ±1.16 & 72.7 ±0.88 & 60.4 ±0.89 & 87.4 ±0.62 & 83.4 ±0.41 & 75.6 ±0.71 & 36.8 ±3.80 & 67.2 ±1.58 & 47.6 ±1.86 & 44.2 ±1.58 & 57.0 ±2.80 & 43.5 ±4.09 \\
            \hline
            \hline
        \end{tabular}
    }
    \caption{\textbf{Comparison of Time and Frequency coordinate maps.} Coordinate maps are inserted in the Resblocks. Test accuracy is reported by question type (Examples for each question type are available in Table \ref{tab:types_of_question}).}
    \label{tab:q_type:coordconv}
\end{table}

The impact of the kind of coordinate maps on each question types is presented in Table \ref{tab:q_type:coordconv}.
To facilitate comparison, all coordinate maps are inserted at the same location (in the first convolution after the feature extractor).
When the network does not include any coordinate maps it reaches only 63.8\%.
Inserting a \emph{Frequency} coordinate map decreases accuracy to 61.7\%.
As hypothesized, \emph{Time} coordinate maps significantly increase the overall accuracy with 79\%.
The accuracy increase for all question types is most notable with questions related to \emph{Absolute position} where the accuracy goes from 41.0\% to 80.2\%.
This is a similar result to \cite{liu2018intriguing} where coordinate maps were proved to help convolutional networks locate objects in visual scenes. 
In the context of a spectro-temporal representation, this ability translates to enhanced temporal localization which naturally helps to answer questions related to position.
Questions related to \emph{Notes} also receive a significant boost from \emph{Time} coordinate maps going from 61.8\% to 73\%.
The fact that \emph{Frequency} coordinate maps decrease performance on questions related to \emph{Notes} is rather surprising since notes are mostly defined by the frequency content at a given point in time.
Furthermore, combining both \emph{Time} and \emph{Frequency} coordinate maps slightly reduces the overall performance when compared to using only \emph{Time} coordinate maps which is in line with previous results.

\section{Results showing Effects of stride size on both CLEAR2 and DAQA'}
\label{sec:small_big_stride}
\begin{table}[H]
    \centering
    %\resizebox{\textwidth}{!}{
        \begin{tabular}{lcccccr}
            \hline
            \hline
            Model   & Nb Parameters & Train acc & Val acc & Test acc & Trainig time \\
            \hline
            \hline
            \multicolumn{2}{l}{On CLEAR2 dataset} & & & \\
            \hline
\NAAQAParallelOptimized - Long stride & 1.68 M & \textbf{95.2 ±0.43} & \textbf{90.5 ±0.28} & \textbf{79.1 ±0.32} & 0 days 02:39:51 \\
\NAAQAParallelOptimized - Short stride & 1.68 M & 93.1 ±0.48 & 89.5 ±0.38 & 77.9 ±0.68 & 0 days 07:00:01 \\
%NAAQA + MALiMo - Big stride & 2.78 M & 93.0 ±1.50 & 88.8 ±0.86 & 77.5 ±0.64 & 0 days 03:39:15.643330 \\
            \hline
            \hline
            \multicolumn{2}{l}{On {\DAQAp} dataset} & & & \\
            \hline
\NAAQAParallelOptimized - Short Stride & 1.68 M & 68.0 ±0.22 & 64.6 ±0.34 & 65.3 ±0.37 & \textbf{3 days 17:27:45} \\
\NAAQAParallelOptimized - Long Stride & 1.68 M & 67.3 ±1.38 & 60.2 ±0.24 & 60.3 ±0.20 & 0 days 07:14:17 \\
%NAAQA - Big Stride & 2.78 M & 67.3 ±1.22 & 64.1 ±0.54 & 64.3 ±0.72 & 0 days 18:10:51.723403 \\
            \hline
            \hline
        \end{tabular}
    %}
    \caption{\textbf{Short stride and Long Stride comparison} The optimized NAAQA on CLEAR2 and DAQA'. The rows are ordered by test accuracy. For CLEAR2, the short stride correspond to 5ms and the long stride is 42.7 ms. For DAQA', the short stride correspond to 10 ms and the long stride is 100 ms.}
    \label{tab:q_type:small_big_stride}
\end{table}
%JR Results reported in Table \ref{tab:q_type:small_big_stride}

\section{Discussion on results with Resnet}
\label{appendix:resnet}
Multiple feature extractors were evaluated in Section \ref{exp:feat_extractor}.
One of them is the Resnet-101 pre-trained on ImageNet (Visual dataset). 
This extractor achieves the lowest of all tested extractors with 62.3\%.
However, it performs quite well with questions related to \emph{brightness} and \emph{loudness} with 83.9\% and 81.9\% respectively.
One possible explanation is that both brightness and loudness are directly related to the amplitude of the ``pixels'' along the frequency axis which may be efficiently encoded by the Resnet101 model.
The \emph{baseline} does not perform as well with questions related to \emph{absolute position} which is somewhat surprising since these questions correspond to a similar pattern matching problem on the time axis instead of the frequency axis.
The \emph{baseline} model also has difficulties with questions related to \emph{notes} (37.8\%).
This might be explained by the fact that a note can be identified by its fundamental frequency and harmonics which can be far apart on the frequency axis.
Visual models are trained to recognize localized features and therefore struggle to recognize notes.
This is a feature that is typical of acoustic signals.


%JR \jer{This part about global position question might be worth keeping in the article.}
It does however perform better with \emph{global position} questions.
This is logical because this type of question refers to an approximate position (beginning, middle, end) which constrain the number of possible answers to 3 instead of 15.




\section{Variability of the input size}
\label{appendix:batching}
Batch normalization has been proven to help regularize the training of neural networks~\cite{IoffeAndSzegedy2015ICMLConditionalBatchNormalization}. 
However, using batch normalization requires all inputs in a batch to have the same dimensions in order to compute the element-wise means and standard deviations. 
Acoustic signals in the CLEAR dataset have variable duration.
To work around this constraint, we padded the spectrograms with zeros so that they all have the same dimensions.
Another solution is to resize all spectrograms to a fixed size using bilinear interpolation as it is commonly done in the visual domain.
From a purely acoustic point of view, we hypothesized that padding spectrograms would preserve the relative time axis between all scenes and would yield better results than resizing.
We revisited this hypothesis by training our best architecture on resized spectrograms. 
Surprisingly, the network performed better by about 1 percentage points when trained on the resized spectrograms.
We do not have a definitive answer as to why we observe this behavior.
It might be due to the fact that padded spectrograms contain less information since a portion of them is filled with zeros. 
The network could also be using the different time resolutions in the resized spectrograms as a cue to cheat the reasoning process.
However, this could also happen when the scenes are padded since the padded section is unique to each scene.
We analyzed the network activations and did not find that the padded section was overly activated.
We leave it up to future work to further analyze this.

\section{Importance of text versus audio modality}
\label{dis:modalities}
%In Section \ref{exp:dataset_size}, we observed that a higher number of questions per scene during training did not improve the test accuracy. 
%This contradicted our hypothesis that increasing the number of questions per scene would increase the performance of the model. 
%It also suggests that the network uses both the scene and question to solve the task without favoring one or the other. 
To validate the fact that NAAQA makes good use of both input modalities (spectrogram and text), the network was trained using only one modality. 
To do so, either all values of the input spectrograms were set to 1 or all questions were set to the \emph{unknown token} during training.
%The results for this experiment are reported on row 2 and 3 of Table \ref{tab:results:clear2}.
No more than 48\% of accuracy on the test set was achieved for either of these scenarios which indicates that the network uses information from both modalities to achieve high performance and that the dataset cannot be solved using only one modality with this architecture. 
This is however much higher than the probability of answering the correct answer by chance ($\frac{1}{57} = 1.75\%$), or by majority vote (7.5\%) introduced in Section \ref{sec:dataset}.
Although we have carefully designed the data set in order to avoid bias, some form of bias is intrinsic in QA problems. For example, an acoustic sequence containing only $n$ elementary sounds automatically disables all counting answers above $n$ regardless which question is asked. Similarly, asking a yes/no question limits the number of possible answers to two, regardless of the acoustic scene. 

%The denominator used in the chance level (57) will, therefore be lower on average. It remains to investigate if our results are consistent with this argument, or if they suggest a residual bias in the dataset. We leave this investigation for future work.


\section{DAQA' missing sounds}
\label{appendix:daqa_missing}
Here is a list of all the missing elementary sounds that were originally in DAQA and that are not in the DAQA' dataset (because of not being anymore accessible on YouTube) : \\
\emph{b000\_20, b000\_3, b000\_4, b000\_5, b000\_6, b001\_11, c001\_13, c001\_14, c001\_15, c001\_16, c001\_17, c001\_18, c001\_19, c001\_20, c003\_9, c004\_10, d001\_1, d001\_9, d002\_19, f001\_19, h001\_10, h001\_11, h001\_12, h001\_13, h001\_14, h001\_15, h001\_19, h001\_2, h001\_3, h001\_4, h001\_5, h001\_6, h001\_7, h001\_8, h001\_9, h002\_10, h002\_11, h002\_12, h002\_8, h002\_9, t000\_14, t000\_15}

\section{Network Optimization}
\label{appendix:optim}

\begin{table}
    \centering
    %\resizebox{0.75\columnwidth}{!}{
        \begin{tabular}{ccccc}
            \hline
            \hline
            Gru (\textbf{G}) & \multicolumn{3}{c}{Overall Accuracy (\%)} & Nb of \\
            Units & Train & Val & Test & Parameters \\
            \hline
           512 & 95.5 ±0.28 & 90.1 ±0.37 & \textbf{79.6 ±0.30} & 1.94 M \\
           256 & 94.3 ±0.51 & \textbf{90.5 ±0.30} & 79.5 ±0.05 & 1.68 M \\
         1,024 & 94.2 ±0.31 & 89.7 ±0.18 & 79.0 ±0.14 & 2.46 M \\
         4,096 & 94.8 ±0.25 & 89.9 ±0.25 & 78.9 ±0.23 & 5.61 M \\
         2,048 & \textbf{95.8 ±0.14} & 90.0 ±0.05 & 78.7 ±0.04 & 3.51 M \\
            \hline
            \hline
        \end{tabular}
    %}
    \caption{\textbf{Impact of the number of GRU text-processing units $G$.} 
    The interleaved extractor is used with hyper-parameters from the initial configuration described in Section \ref{exp:initial_config} except for $G$.
  %JR  The row marked with * corresponds to the initial value for $G$. 
    The number of GRU unit has a strong impact on the number of parameters. 
    Setting $G=512$ actually increases accuracy while reducing the number of parameters by a factor of $\sim$2.8. The rows are ordered by test accuracy.}
    \label{tab:gru_reduction}
\end{table}



\begin{table}
    \centering
    %\resizebox{0.6\columnwidth}{!}{
        \begin{tabular}{cccccc}
            \hline
            \hline
            Nb (\textbf{J}) & Nb Filter (\textbf{M}) & \multicolumn{3}{c}{Overall Accuracy (\%)} & Nb of \\
            Resblock & in Resblock & Train & val & Test & Parameters \\
            \hline
           4 & 128 & \textbf{94.9 ±0.91} & \textbf{89.9 ±0.39} & \textbf{79.1 ±0.56} & \textbf{1.94 M} \\
           3 & 128 & 95.0 ±0.67 & 89.4 ±0.42 & 78.4 ±0.25 & 1.64 M \\
           2 & 128 & 93.6 ±0.40 & 86.9 ±0.61 & 77.3 ±0.88 & 1.35 M \\
           4 & 64 & 92.8 ±0.95 & 87.6 ±0.98 & 77.0 ±0.66 & 1.11 M \\
           3 & 64 & 91.8 ±1.36 & 86.2 ±0.77 & 76.4 ±0.65 & 1.01 M \\
           2 & 64 & 90.8 ±0.75 & 84.5 ±0.64 & 75.0 ±0.63 & 0.90 M \\
           4 & 32 & 88.1 ±1.35 & 83.1 ±1.08 & 73.6 ±1.18 & 0.82 M \\
           3 & 32 & 86.3 ±1.39 & 80.6 ±1.54 & 71.5 ±1.54 & 0.78 M \\
           2 & 32 & 84.4 ±1.36 & 76.8 ±2.02 & 68.4 ±1.59 & 0.74 M \\
           1 & 128 & 89.0 ±1.80 & 75.3 ±2.65 & 67.2 ±2.43 & 1.05 M \\
           1 & 64 & 84.3 ±4.61 & 69.6 ±4.61 & 62.1 ±3.41 & 0.79 M \\
           1 & 32 & 67.0 ±3.58 & 57.3 ±2.07 & 52.9 ±1.50 & 0.69 M \\
            \hline
            \hline
        \end{tabular}
    %}
    \caption{\textbf{Impact of reducing the number of Resblock $J$ and the number of filters $M$ in each Resblocks.} 
    The interleaved extractor is used with hyper-parameters from the initial configuration described in Section \ref{exp:initial_config} except for $J$, $M$, $C=256$, $H=1024$ and $G=512$.
    With $J=4$ and $M=64$, the network reaches great accuracy with only 0.67M parameters (vs 5.61M for the initial configuration).
    The accuracy drops when $J<3$ and $M=32$.
    The configuration $J=3$ and $M=128$ get stuck in local minimums often which explain the large STD. The rows are
ordered by test accuracy
    }
    \label{tab:resblocks_reduction}
\end{table}

\iffalse
\begin{table}
    \centering
    %\resizebox{0.95\columnwidth}{!}{
        \begin{tabular}{cccccc}
            \hline
            \hline
            Nb (\textbf{K}) & Projection (\textbf{P}) & \multicolumn{3}{c}{Accuracy (\% ± 0.60)} & Nb of \\
            Block & Size & Train & val & Test & Parameters \\
            \hline
3 & 32 & 93.7 ±0.34 & 91.5 ±0.03 & 91.5 ±0.15 & $\sim$0.81 M \\
3 & 64 & 93.7 ±0.04 & 91.0 ±0.26 & 91.1 ±0.04 & $\sim$0.83 M \\
3 & 128 & 93.1 ±0.24 & 91.0 ±0.66 & 91.1 ±0.36 & $\sim$0.87 M \\
3 & -- & 93.5 ±0.30 & 91.1 ±0.24 & 90.8 ±0.29 & $\sim$0.81 M \\
2 & -- & 92.9 ±0.39 & 89.9 ±0.13 & 90.0 ±0.13 & $\sim$0.80 M \\
2 & 32 & 92.9 ±0.72 & 89.7 ±0.62 & 89.9 ±0.55 & $\sim$0.81 M \\
2 & 128 & 91.9 ±1.80 & 89.5 ±0.75 & 89.5 ±1.03 & $\sim$0.87 M \\
2 & 64 & 91.9 ±1.14 & 89.4 ±0.57 & 89.4 ±0.58 & $\sim$0.83 M \\
4 & 32 & 93.4 ±0.47 & 86.9 ±2.43 & 83.1 ±0.07 & $\sim$0.83 M \\
4 & 64 & 89.0 ±0.00 & 81.6 ±0.00 & 80.8 ±0.00 & $\sim$0.86 M \\
4 & -- & 91.3 ±2.00 & 83.5 ±6.44 & 79.9 ±4.09 & $\sim$0.85 M \\
4 & 128 & 88.2 ±2.37 & 77.3 ±2.70 & 74.8 ±2.62 & $\sim$0.90 M \\
            \hline
            \hline
        \end{tabular}
    %}
    \caption{\textbf{Impact of the number of blocks $K$ in the parallel feature extractor and its projection size $P$.} 
    The interleaved extractor is used with the hyper-parameters {$J=4$}, {$M=64$}, {$C=256$}, {$H=1024$}, {$G=512$}.
    More blocks in the extractor results in more downsampling of the feature maps.
    Too much downsampling ($K=4$) negatively affects accuracy.}
    \label{tab:extractor_reduction}
\end{table}
\fi
Tables \ref{tab:gru_reduction} and  \ref{tab:resblocks_reduction} report the intermediate results of the NAAQA network complexity study on CLEAR2.
