# Supplementary material for: NAAQA: A Neural Architecture for Acoustic Question Answering
Source: arXiv:2106.06147 source file (2024-01-12)
Supplement: Supplementary file 2 [file supplementary.tex]

\documentclass[journal,compsoc]{IEEEtran}
\pdfoutput=1

\usepackage{amsmath}
\usepackage{multirow}
\usepackage{siunitx}
\usepackage{graphicx}
\usepackage{stfloats}
\usepackage{booktabs}
\usepackage{caption}
\usepackage{subcaption}
\usepackage{textcomp}
\usepackage[hidelinks]{hyperref}
\usepackage{float}
\usepackage[backend=biber,bibstyle=ieee,citestyle=numeric-comp,maxbibnames=2,minbibnames=1,mincitenames=1,maxcitenames=2,doi=false,isbn=false, url=false]{biblatex}
\addbibresource{references2.bib}
\usepackage{xcolor}
\usepackage{xspace}
\newcommand{\gs}[1]{{\color{blue}\textbf{GS:} #1}}
\newcommand{\jer}[1]{{\color{red}(\textbf{JER:} #1)}}
\newcommand{\jean}[1]{{\color{brown}(\textbf{JEAN:} #1)}}
%\renewcommand{\gs}[1]{}
%\renewcommand{\jer}[1]{}
%\renewcommand{\jean}[1]{}

\renewcommand{\appendixname}{Supplementary}

% correct bad hyphenation here
%\hyphenation{op-tical net-works semi-conduc-tor}

% useful strings
\newcommand{\DAQAp}{DAQA$^\prime$\xspace}
\newcommand{\VisualFiLM}{\textbf{\texttt{Visual FiLM Resnet101}}\xspace}
\newcommand{\NAAQATwoDConv}{\textbf{\texttt{NAAQA 2D Conv}}\xspace}
\newcommand{\NAAQAParallel}{\textbf{\texttt{NAAQA Parallel}}\xspace}
\newcommand{\NAAQAInterleavedTime}{\textbf{\texttt{NAAQA Interleaved Time}}\xspace}
\newcommand{\NAAQAInterleavedFreq}{\textbf{\texttt{NAAQA Interleaved Freq}}\xspace}
\newcommand{\NAAQAParallelOptimized}{\textbf{\texttt{Optimized NAAQA Parallel}}\xspace}
\newcommand{\NAAQATwoDConvOptimized}{\textbf{\texttt{Optimized NAAQA 2D Conv}}\xspace}
\newcommand{\MALiMo}{\textbf{\texttt{MALiMo ctrl}}\xspace}

% Instructions:
% 1) compile with this commented out (this will generate all auxiliary files)
% 2) compile with this active (to output only supplementary material)
\includeonly{appendix}

\begin{document}
\include{introduction}
\include{dataset}
\include{methods}
\include{experiments}
%\input{discussion}
\include{conclusion}

\begin{appendices}
\include{appendix}
\end{appendices}
\end{document}
